# Supplementary material for: Opportunities for Price Manipulation by Aggregators in Electricity Markets
Source: arXiv:1606.06510 source file (2016-06-21)
Supplement: Supplementary file 1 [file appendix.tex]

\subsection{Proof of Theorem \ref{prop: uniform}}

		When there is no congestion in the network, $\mathbf{G'}^T = \mathbf{0}$, the following relationship holds
		\[ \lambda\mathbbm{1} = \mathbf{c} + \amax - \amin, 
		\]
		Hence the location marginal prices are uniform and all equal to $\lambda$. 
		Furthermore, now the dual problem \eqref{eqn: dual_obj} can be seen as adjusting $\mathbf{c}$ upwards and downwards so that it becomes a level vector $\lambda\mathbbm{1}$, specifically, $\dpu_i$ $\dpl_i$ is the unit cost of upward and downward adjustment on the $i^{th}$ coordinate of $\mathbf{c}$. 
		 
		 Let $L(y)$ be the objective value of \eqref{eqn: dual_obj} when we fix $\lambda = y$, then $\lambda = \arg\min_y L(y)$. It is easy to check that $\lambda \in [c_{\pi(N)}, c_{\pi(1)}]$ since $L(y) > L(\cpo)$ for all $y > \cpo$, and $L(y) > L(c_{\pi(N)})$ for all $y < c_{\pi(N)}$. 
		 
		 Since both $\amax \ge \mathbf{0}$ and $\amin  \ge \mathbf{0}$, 
		 we have $\amax = (y\mathbbm{1} - \vct{c})_+ $ and $\amin = (y\mathbbm{1} - \vct{c})_-$\footnote{We denote $\vct{a} = (\vct{x})_+$ when $a_i = x_i$ for all $x_i \ge 0$, and $a_i = 0$ otherwise. Similarly, denote $\vct{a} = (\vct{x})_-$ when $a_i = -x_i$ for all $x_i <0$ and $a_i =0$ otherwise.}. %For any $y$, let $h(y) = \arg\min_i \{ c_{\pi(i)} > y\}$ the coordinate of smallest $c_{\pi(i)}$ that is greater than $y$. 
		 Hence we have 
 		\begin{align}
			\label{eqn: l_y}
 			& L(y) = \langle \dpu, (y\mathbbm{1} - \vct{c})_+ \rangle - \langle \dpl, (y\mathbbm{1} - \vct{c})_- \rangle \\
 				 = & \begin{dcases}
				 \sum_{j=1}^{i} |\dpl_{\pi(j)}| (\cpj - y) + &  \sum_{j = i + 1}^N \dpu_{\pi(j)} (y - c_{\pi(j)}),\\
                 & \text{ if } y \in (c_{\pi(i+1)}, \cpi); \\
				 \sum_{j=1}^{i-1} |\dpl_{\pi(j)}| (\cpj - y) + &  \sum_{j = i + 1}^N \dpu_{\pi(j)} (y - c_{\pi(j)}), \\
                 & \text{ if } y = \cpi.
				 \end{dcases} \notag
  		\end{align} 
		 The subgradient of $L(y)$ is 
		 \begin{align*}
		 \frac{\partial L(y)}{\partial y} = \sum_{j=i+1}^N \dpu_{\pi(j)} - \sum_{j=1}^i |\dpl_{\pi(j)}|, 
		 \end{align*}
		 when $y \in (c_{\pi(i+1)}, \cpi)$. When $y = \cpi$, the subgradient $\partial L(y) / \partial y  $ is the following set:
		 \begin{align*}
		 \left[ \sum_{j=i+1}^N \dpu_{\pi(j)} - \sum_{j=1}^i \left|\dpl_{\pi(j)}\right|, \  \sum_{j=i}^N \dpu_{\pi(j)} - \sum_{j=1}^{i-1} \left|\dpl_{\pi(j)}\right| \right].
		 \end{align*}
		 The subgradient is increasing with respect to $y$, hence $L(y)$ is a convex function. We can derive the optimal $\lambda$ by investigating the first order condition, which can be divided into two cases:
		 
		 Case 1, if $\sum_{j=i}^N \dpu_{\pi(j)} - \sum_{j=1}^{i-1} |\dpl_{\pi(j)}| > 0$ and $ \sum_{j=i+1}^N \dpu_{\pi(j)} - \sum_{j=1}^i |\dpl_{\pi(j)}| <0$ for some $i \in \{1, \ldots, N\}$, then $ 0 \in \frac{\partial L(y)}{\partial y} \Bigr|_{y = \cpi}$, hence $\lambda = \arg\min_y L(y) = \cpi$. 
		 
		 Case 2, if $\sum_{j=i+1}^N \dpu_{\pi(j)} - \sum_{j=1}^i |\dpl_{\pi(j)}| = 0 $ for some $i \in \{1, \ldots, N\}$, then $\frac{\partial L(y)}{\partial y} = 0$ for all $y \in (c_{\pi(i+1)}, \cpi)$, and furthermore, $0 \in \frac{\partial L(y)}{\partial y} \Bigr|_{y = \cpi}$, and $ 0 \in \frac{\partial L(y)}{\partial y} \Bigr|_{y = c_{\pi(i+1)}}$, hence the objective attains minimum value for all $\lambda \in [c_{\pi(i+1)}, \cpi]$.

	\subsection{Proof of Proposition \ref{prop: tight_constraint}}
		As $\Delta \bar{p}_i \ge 0, \Delta \underline{p}_i \le 0$, the dual objective function \eqref{eqn: dual_obj} is always nonnegative for all $\alpha_{\max}\ge 0$ and $\alpha_{\min} \ge 0$. However, if $\eqref{eqn: tight_constraint}$ holds, then take $\lambda = x_1 - x_2$, and take $\mu = x_{3:N}$, hence \eqref{eqn: tight_constraint} implies that $\lambda\mathbbm{1} + \mathbf{G'}^T \mu = \mathbf{c}$, hence \eqref{eqn: equality_cons} can be satisfied with $\alpha_{\max} = \alpha_{\min} = \mathbf{0},$ and the dual objective function \eqref{eqn: dual_obj} obtained its minimum possible value. 

\subsection{Proof of Lemma \ref{lemma: tree_simplify}}
Let node $i$ and node $j$ be connected by an uncongested line $l$, without loss of generality, we can assume node $j$ as the reference node and $G_j$, the $j^{th}$ column of $\mtx{G}$ is $\vct{0}$. Otherwise, we can define an alternate shift factor matrix $\mtx{H} = \mtx{G} - G_j\mathbbm{1}^T$. For any marginal flow $\Delta p$ such that $\sum_i \Delta p_i = 0$, the flow on each line $l$ is equivalent since $\sum_i H_{l,i}  \Delta p_i = \sum_i G_{l, i}\Delta p_i - G_{l, j} (\sum_i \Delta p_i) = \sum_i G_{l, i}\Delta p_i$. 

For $G_i$, the only positive entry is $G_{l, i}$, since if for any $l'$ such that $G_{l', i} \ne 0$, it means there are multiple paths of power flow from $i$ to $j$, contradicting the fact that the network is acyclic. 

Since $l$ is uncongested, we have $G'_{l, i} = 0$ in the congestion pattern matrix, hence $G'_i = \vct{0} = G'_j$. Therefore the locational marginal price $\lambda_i = \lambda + G_i'^T \mu = \lambda = \lambda_j$. Iterating this argument, we can conclude that all nodes connected by uncongested lines must have the same LMP. 

\subsection{Proof of Lemma \ref{lemma: tree_congestion}}
By Lemma \ref{lemma: tree_simplify}, it suffices to prove the result for a pair of nodes $i, j$ connected by a congested line $l$, where the line flow on $l$ is from $i$ to $j$. Without loss of generality, assume that $j$ is the reference node. Hence the only nonzero entry in $G_i$ is $G_{l, i}$. Moreover, since congestion direction is from $i$ to $j$, if $G_{l, i} > 0$, then $l$ is positively congested, i.e., $l \in \mathcal{C}_+$. 
If $G_{l, i} <0$, then $l$ is negatively congested, i.e., $l \in \mathcal{C}_-$. In both cases, by definition of the congestion pattern matrix, $G'_{i} < \vct{0} = G'_j$. Therefore $\lambda_i = \lambda + G'^T_i \mu \le \lambda = \lambda_j$.

\subsection{Proof of Lemma \ref{lemma: mesh_congestion}}
Without loss of generality, we can assume that $j$ is the reference bus, $G_j = \vct{0}$. If the condition given in the lemma is true, then for each congested $l$, if $G_{i,j} >0$, it is opposed to the direction of sending power from $j$ to $i$, hence it must be negatively congested, i.e., $l \in \mathcal{C}_-$; if $G_{l, i}<0$, it is in the direction of sending power from $j$ to $i$, hence it must be positively congested, i.e., $l \in \mathcal{C}_+$. Hence by the definition of $\mtx{G}' = \mathrm{diag}(\mathbbm{1}_- - \mathbbm{1}_+) G$, we have $G_i > 0$. Therefore $\lambda_i = \lambda + G_i^T \mu \ge \lambda = \lambda_j$.
